# Supplementary material for: Monotonicity and convergence of two-relaxation-times lattice Boltzmann schemes for a non-linear conservation law
Source: arXiv:2501.07934 source file (2025-04-30)
Supplement: Supplementary file 1 [file 2025_Aregba-Bellotti_TRT_LBM_Supplementary.pdf]

# SUPPLEMENTARY MATERIALS: MONOTONICITY AND CONVERGENCE OF TWO-RELAXATION-TIMES LATTICE BOLTZMANN SCHEMES FOR A NON-LINEAR CONSERVATION LAW

DENISE AREGBA-DRIOLLET* AND THOMAS BELLOTTI†

**SM1. Proof of Proposition 3.9.** The monotonicity conditions for the equilibria read

$$\mathscr{L}_1 \geq 0 \qquad \text{and} \qquad \max_{\mathsf{u}\in[-u_\infty, u_\infty]} \Big| \sum_{k=1}^{d} \mathscr{N}_{2\ell,k}\varphi_k'(\mathsf{u}) \Big| \leq \mathscr{L}_{2\ell}, \qquad \ell \in [\![1, W]\!]. \tag{SM1.1}$$

Let us start by the sufficient part of the claim. If the conditions in Proposition 3.3 are met, that is we have $(\omega_{\mathsf{s}}, \omega_{\mathsf{a}}) \in \mathcal{M}$, the first inequality in (SM1.1) is fulfilled, whatever the sign of $\omega_{\mathsf{a}} - \omega_{\mathsf{s}}$, since $\max(0, \omega_{\mathsf{s}} - 1) \geq 0$ and $\omega_{\mathsf{s}} > 0$. For similar reasons, we have that for any $\ell \in [\![1, W]\!]$

$$\begin{aligned}
\mathscr{L}_{2\ell} &\geq \frac{\omega_{\mathsf{a}}}{\omega_{\mathsf{s}}} \max_{\mathsf{u}\in[-u_\infty, u_\infty]} \Big| \sum_{k=1}^{d} \mathscr{N}_{2\ell,k}\varphi_k'(\mathsf{u}) \Big| - \frac{1}{2\omega_{\mathsf{s}}} \min(2 - \omega_{\mathsf{s}} - \omega_{\mathsf{a}}, 0, \omega_{\mathsf{a}} - \omega_{\mathsf{s}}) \\
&\geq \frac{\omega_{\mathsf{a}}}{\omega_{\mathsf{s}}} \max_{\mathsf{u}\in[-u_\infty, u_\infty]} \Big| \sum_{k=1}^{d} \mathscr{N}_{2\ell,k}\varphi_k'(\mathsf{u}) \Big| \geq 0, \qquad \text{(SM1.2)}
\end{aligned}$$

hence whenever $\omega_{\mathsf{a}} \geq \omega_{\mathsf{s}}$, the second inequality in (SM1.1) is also satisfied. This includes the BGK case studied in [SM1].

The case $\omega_{\mathsf{a}} < \omega_{\mathsf{s}}$ is handled by contradiction. Assume that equilibria are not monotone, which means that there exists $\tilde{\ell} \in [\![1, W]\!]$ and $\mathsf{u} \in [-u_\infty, u_\infty]$ such that

$$\Big| \sum_{k=1}^{d} \mathscr{N}_{2\tilde{\ell},k}\varphi_k'(\mathsf{u}) \Big| > \mathscr{L}_{2\tilde{\ell}}.$$

For the same link $\tilde{\ell}$, the conditions of Proposition 3.3 give:

$$\begin{aligned}
\omega_{\mathsf{a}}\mathscr{L}_{2\tilde{\ell}} < \omega_{\mathsf{a}} \Big| \sum_{k=1}^{d} \mathscr{N}_{2\tilde{\ell},k}\varphi_k'(\mathsf{u}) \Big| &\leq \omega_{\mathsf{s}}\mathscr{L}_{2\tilde{\ell}} + \tfrac{1}{2}\min(2 - \omega_{\mathsf{s}} - \omega_{\mathsf{a}}, 0, \omega_{\mathsf{a}} - \omega_{\mathsf{s}}) \\
&\leq \omega_{\mathsf{s}}\mathscr{L}_{2\tilde{\ell}} + \tfrac{1}{2}(\omega_{\mathsf{a}} - \omega_{\mathsf{s}}).
\end{aligned}$$

The two outermost inequalities in the previous expression entail $(\omega_{\mathsf{a}} - \omega_{\mathsf{s}})\mathscr{L}_{2\tilde{\ell}} < \frac{1}{2}(\omega_{\mathsf{a}} - \omega_{\mathsf{s}})$, hence, since $\omega_{\mathsf{a}} - \omega_{\mathsf{s}} < 0$, we obtain $\mathscr{L}_{2\tilde{\ell}} > \frac{1}{2}$. By consistency, *cf.* (3.4), we have that

$$1 = \mathscr{L}_1 + 2\sum_{\ell=1}^{W} \mathscr{L}_{2\ell} = \mathscr{L}_1 + 2\mathscr{L}_{2\tilde{\ell}} + 2\sum_{\substack{\ell=1 \\ \ell\neq\tilde{\ell}}}^{W} \mathscr{L}_{2\ell} > 1 + 2\sum_{\substack{\ell=1 \\ \ell\neq\tilde{\ell}}}^{W} \mathscr{L}_{2\ell},$$

*Université de Bordeaux, CNRS, Bordeaux INP, IMB, UMR 5251, 33400 Talence, France.

†Université Paris-Saclay, CNRS, CentraleSupélec, Laboratoire EM2C & Fédération de Mathématiques de CentraleSupélec, 91190, Gif-sur-Yvette, France.



*This manuscript is for review purposes only.*

where we have used that $\mathscr{L}_1 \geq 0$ and $\mathscr{L}_{2\tilde{\ell}} > \frac{1}{2}$. This implies that

$$\sum_{\substack{\ell=1\\ \ell\neq\tilde{\ell}}}^{W} \mathscr{L}_{2\ell} < 0: \qquad \text{contradiction with (SM1.2)!}$$

We then apply [SM1, Proposition 2.1], which states that in the BGK case, upon having monotone equilibria (which we now have), the condition (3.11) is necessary (maximal character) and sufficient to have monotonicity of the relaxation operator. We have therefore proved the necessary part, for monotone equilibria entail $\varnothing \neq \{(\omega, \omega) \ : \ \omega \in \mathcal{M}_{\text{BGK}}\} \subset \mathcal{M}$, thus $\mathcal{M} \neq \varnothing$.

**SM2. Proof of Proposition 3.10.** We start by preliminary computations giving expressions analogous to [SM1, Eq. (25) and (26)]. For the first row of the Jacobian

$$\partial_{\mathsf{f}_1}\mathcal{R}_1(\mathsf{f}_1, \dots, \mathsf{f}_q) = 1 - \omega_{\mathsf{s}}\Big(1 - \frac{\mathrm{d}f_1^{\text{eq}}(\mathsf{u})}{\mathrm{d}\mathsf{u}}\Big) \geq 0, \tag{SM2.1}$$
$$\partial_{\mathsf{f}_i}\mathcal{R}_1(\mathsf{f}_1, \dots, \mathsf{f}_q) = \omega_{\mathsf{s}}\frac{\mathrm{d}f_1^{\text{eq}}(\mathsf{u})}{\mathrm{d}\mathsf{u}} \geq 0,$$

for $i \in [\![2, q]\!]$, which is as in the BGK context. Let $\ell \in [\![1, W]\!]$ be any link, then

$$\partial_{\mathsf{f}_{2\ell}}\mathcal{R}_{2\ell} = \overbrace{1 - \omega_{\mathsf{s}}\Big(1 - \frac{\mathrm{d}f_{2\ell}^{\text{eq}}(\mathsf{u})}{\mathrm{d}\mathsf{u}}\Big)}^{\text{BGK-part}} + \overbrace{\tfrac{1}{2}(\omega_{\mathsf{s}} - \omega_{\mathsf{a}})\Big(1 - 2\sum_{k=1}^{d}\mathscr{N}_{2\ell,k}\varphi_k'(\mathsf{u})\Big)}^{\text{TRT-part}} \geq 0, \tag{SM2.2}$$
$$\partial_{\mathsf{f}_{2\ell+1}}\mathcal{R}_{2\ell+1} = 1 - \omega_{\mathsf{s}}\Big(1 - \frac{\mathrm{d}f_{2\ell+1}^{\text{eq}}(\mathsf{u})}{\mathrm{d}\mathsf{u}}\Big) + \tfrac{1}{2}(\omega_{\mathsf{s}} - \omega_{\mathsf{a}})\Big(1 + 2\sum_{k=1}^{d}\mathscr{N}_{2\ell,k}\varphi_k'(\mathsf{u})\Big) \geq 0.$$

Also

$$\partial_{\mathsf{f}_{2\ell+1}}\mathcal{R}_{2\ell} = \omega_{\mathsf{s}}\frac{\mathrm{d}f_{2\ell}^{\text{eq}}(\mathsf{u})}{\mathrm{d}\mathsf{u}} - \tfrac{1}{2}(\omega_{\mathsf{s}} - \omega_{\mathsf{a}})\Big(1 + 2\sum_{k=1}^{d}\mathscr{N}_{2\ell,k}\varphi_k'(\mathsf{u})\Big) \geq 0, \tag{SM2.3}$$
$$\partial_{\mathsf{f}_{2\ell}}\mathcal{R}_{2\ell+1} = \omega_{\mathsf{s}}\frac{\mathrm{d}f_{2\ell+1}^{\text{eq}}(\mathsf{u})}{\mathrm{d}\mathsf{u}} - \tfrac{1}{2}(\omega_{\mathsf{s}} - \omega_{\mathsf{a}})\Big(1 - 2\sum_{k=1}^{d}\mathscr{N}_{2\ell,k}\varphi_k'(\mathsf{u})\Big) \geq 0.$$

We now proceed by contradiction. Assume that $\omega_{\mathsf{s}} = 2$. From the first inequality in (SM2.1), we obtain

$$\frac{\mathrm{d}f_1^{\text{eq}}(\mathsf{u})}{\mathrm{d}\mathsf{u}} \geq \tfrac{1}{2}.$$

Using (SM2.2), we gain

$$2\frac{\mathrm{d}f_{2\ell}^{\text{eq}}(\mathsf{u})}{\mathrm{d}\mathsf{u}} + \tfrac{1}{2}(2 - \omega_{\mathsf{a}})\Big(1 - 2\sum_{k=1}^{d}\mathscr{N}_{2\ell,k}\varphi_k'(\mathsf{u})\Big) \geq 1,$$
$$2\frac{\mathrm{d}f_{2\ell+1}^{\text{eq}}(\mathsf{u})}{\mathrm{d}\mathsf{u}} + \tfrac{1}{2}(2 - \omega_{\mathsf{a}})\Big(1 + 2\sum_{k=1}^{d}\mathscr{N}_{2\ell,k}\varphi_k'(\mathsf{u})\Big) \geq 1,$$

thus summing

$$\frac{\mathrm{d}f_{2\ell}^{\mathrm{eq}}(\mathsf{u})}{\mathrm{d}\mathsf{u}} + \frac{\mathrm{d}f_{2\ell+1}^{\mathrm{eq}}(\mathsf{u})}{\mathrm{d}\mathsf{u}} \geq \frac{\omega_{\mathsf{a}}}{2}.$$

Recall that—by consistency (3.4)—we have that

$$\text{(SM2.4)} \qquad \sum_{i=1}^{q} \frac{\mathrm{d}f_{i}^{\mathrm{eq}}(\mathsf{u})}{\mathrm{d}\mathsf{u}} = 1 \geq \tfrac{1}{2}(1+\omega_{\mathsf{a}}W), \qquad \text{which enforces} \qquad \omega_{\mathsf{a}} \leq \frac{1}{W}.$$

Now, consider (SM2.3). Summing these inequalities gives

$$\frac{\mathrm{d}f_{2\ell}^{\mathrm{eq}}(\mathsf{u})}{\mathrm{d}\mathsf{u}} + \frac{\mathrm{d}f_{2\ell+1}^{\mathrm{eq}}(\mathsf{u})}{\mathrm{d}\mathsf{u}} \geq 1 - \frac{\omega_{\mathsf{a}}}{2}.$$

Through the same remark as before, we gain

$$\text{(SM2.5)} \qquad \sum_{i=1}^{q} \frac{\mathrm{d}f_{i}^{\mathrm{eq}}(\mathsf{u})}{\mathrm{d}\mathsf{u}} = 1 \geq \tfrac{1}{2} + \Big(1 - \frac{\omega_{\mathsf{a}}}{2}\Big)W, \qquad \text{which enforces} \qquad \omega_{\mathsf{a}} \geq 2 - \frac{1}{W}.$$

Notice that (SM2.4) and (SM2.5) are mutually exclusive, unless $W = 1$ and $\omega_{\mathsf{a}} = 1$. This case can only happen when $d = 1$: the monotonicity conditions from Proposition 3.3 become, using the constraint (3.4)

$$\mathscr{L}_2 \leq \tfrac{1}{4}, \qquad |\mathscr{N}_2| \max_{\mathsf{u}\in[-u_\infty, u_\infty]} |\varphi'(\mathsf{u})| \leq 2\mathscr{L}_2 - \tfrac{1}{2},$$

which entails that either $\mathscr{N}_2 = 0$ or $\max_{\mathsf{u}\in[-u_\infty, u_\infty]} |\varphi'(\mathsf{u})| = 0$. Both correspond to the trivial case of constant flux $\varphi$: contradiction!

Assume that $\omega_{\mathsf{a}} = 2$. From the first inequality in (SM2.1)

$$\frac{\mathrm{d}f_{1}^{\mathrm{eq}}(\mathsf{u})}{\mathrm{d}\mathsf{u}} \geq 0.$$

Consider the inequalities in (SM2.2)

$$1 - \omega_{\mathsf{s}} + \omega_{\mathsf{s}} \frac{\mathrm{d}f_{2\ell}^{\mathrm{eq}}(\mathsf{u})}{\mathrm{d}\mathsf{u}} + \tfrac{1}{2}(\omega_{\mathsf{s}} - 2)\Big(1 - 2\sum_{k=1}^{d} \mathscr{N}_{2\ell,k}\varphi_k'(\mathsf{u})\Big) \geq 0,$$

$$1 - \omega_{\mathsf{s}} + \omega_{\mathsf{s}} \frac{\mathrm{d}f_{2\ell+1}^{\mathrm{eq}}(\mathsf{u})}{\mathrm{d}\mathsf{u}} + \tfrac{1}{2}(\omega_{\mathsf{s}} - 2)\Big(1 + 2\sum_{k=1}^{d} \mathscr{N}_{2\ell,k}\varphi_k'(\mathsf{u})\Big) \geq 0.$$

Summing them:

$$\frac{\mathrm{d}f_{2\ell}^{\mathrm{eq}}(\mathsf{u})}{\mathrm{d}\mathsf{u}} + \frac{\mathrm{d}f_{2\ell+1}^{\mathrm{eq}}(\mathsf{u})}{\mathrm{d}\mathsf{u}} \geq 1.$$

The usual procedure gives

$$\sum_{i=1}^{q} \frac{\mathrm{d}f_{i}^{\mathrm{eq}}(\mathsf{u})}{\mathrm{d}\mathsf{u}} = 1 \geq W, \qquad \text{which enforces} \qquad W = 1.$$

Again, this can happen only in the $d = 1$ case. Considering the first equation in (SM2.1), we gain

$$\frac{\mathrm{d}f_1^{\mathrm{eq}}(\mathsf{u})}{\mathrm{d}\mathsf{u}} \geq 1 - \frac{1}{\omega_{\mathsf{s}}},$$

therefore—as usual

$$\frac{\mathrm{d}f_1^{\mathrm{eq}}(\mathsf{u})}{\mathrm{d}\mathsf{u}} + \frac{\mathrm{d}f_2^{\mathrm{eq}}(\mathsf{u})}{\mathrm{d}\mathsf{u}} + \frac{\mathrm{d}f_3^{\mathrm{eq}}(\mathsf{u})}{\mathrm{d}\mathsf{u}} = 1 \geq 2 - \frac{1}{\omega_{\mathsf{s}}}, \qquad \text{which enforces} \qquad \omega_{\mathsf{s}} \leq 1.$$

Now, the monotonicity conditions from proposition 3.3 read

$$\omega_{\mathsf{s}}(1 - 2\mathscr{L}_2) \geq \max(0, \omega_{\mathsf{s}} - 1) = 0, \qquad |\mathscr{N}_2| \max_{\mathsf{u}\in[-u_\infty, u_\infty]} |\varphi'(\mathsf{u})| \leq -\frac{\omega_{\mathsf{s}}}{4}(1 - 2\mathscr{L}_2).$$

This entails that either $\mathscr{N}_2 = 0$ or $\max_{\mathsf{u}\in[-u_\infty,u_\infty]} |\varphi'(\mathsf{u})| = 0$. Both correspond to the trivial case of constant flux $\varphi$: contradiction!

**SM3. Proof of Proposition 3.11.** Using Proposition 3.9, we know that $\varnothing \neq \{(\omega, \omega) \text{ s.t. } \omega \in \mathcal{M}_{\mathrm{BGK}}\} \subset \mathring{\mathcal{M}}$. Assume that $\{(\omega, \omega) \text{ s.t. } \omega \in \mathcal{M}_{\mathrm{BGK}}\} \subset \partial\mathcal{M}$. Since $\mathcal{M}$ is a convex polytope, from (3.6), we know that there exist $\ell \in [\![1, W]\!]$ such that

$$\omega \max_{\mathsf{u}\in[-u_\infty,u_\infty]} \Big|\sum_{k=1}^{d} \mathscr{N}_{2\ell,k}\varphi_k'(\mathsf{u})\Big| = \omega\mathscr{L}_{2\ell}, \tag{SM3.1}$$

or there exist $\ell \in [\![1, W]\!]$ such that

$$\omega \max_{\mathsf{u}\in[-u_\infty,u_\infty]} \Big|\sum_{k=1}^{d} \mathscr{N}_{2\ell,k}\varphi_k'(\mathsf{u})\Big| = \omega\mathscr{L}_{2\ell} + 1 - \omega, \tag{SM3.2}$$

for every $\omega \in \mathcal{M}_{\mathrm{BGK}}$.

Assume that we are in the case where (SM3.1) holds. This equation entails that either $\omega = 0$, which is not possible, or that $\max_{\mathsf{u}\in[-u_\infty,u_\infty]} |\sum_{k=1}^{k=d} \mathscr{N}_{2\ell,k}\varphi_k'(\mathsf{u})| = \mathscr{L}_{2\ell}$. This case may or may not take place according to the choice of parameters. Assume it does. Take $\omega \in \mathcal{M}_{\mathrm{BGK}}$ and assume that $(\omega_{\mathsf{s}}, \omega_{\mathsf{a}}) = (\omega, \omega + \delta) \in \mathcal{M}$, with $\delta > 0$. This gives that

$$-\delta\mathscr{L}_{2\ell} + \tfrac{1}{2}\min(2 - 2\omega - \delta, 0, \delta) \geq 0.$$

The first term in the sum is strictly negative ($\mathscr{L}_{2\ell} \neq 0$, otherwise things are trivial) and the second one is non-positive: contradiction with the fact of having $\mathcal{M} \cap \{(\omega_{\mathsf{s}}, \omega_{\mathsf{a}}) \text{ s.t. } \omega_{\mathsf{a}} > \omega_{\mathsf{s}}\} \neq \varnothing$.

Assume that we are in the case where (SM3.2) holds. There is only one value of $\omega$, given by

$$\begin{aligned}\omega &= \frac{1}{1 - \mathscr{L}_{2\ell} + \max_{\mathsf{u}\in[-u_\infty,u_\infty]} |\sum_{k=1}^{k=d} \mathscr{N}_{2\ell,k}\varphi_k'(\mathsf{u})|}\\ &\leq \min\Big(\frac{1}{1 - \mathscr{L}_1}, \frac{1}{1 - \mathscr{L}_2 + \max_{\mathsf{u}\in[-u_\infty,u_\infty]} |\sum_{k=1}^{k=d} \mathscr{N}_{2,k}\varphi_k'(\mathsf{u})|},\\ &\qquad \dots, \frac{1}{1 - \mathscr{L}_{2W} + \max_{\mathsf{u}\in[-u_\infty,u_\infty]} |\sum_{k=1}^{k=d} \mathscr{N}_{2W,k}\varphi_k'(\mathsf{u})|}\Big),\end{aligned}$$

so that

$$\frac{1}{1-\mathscr{L}_{2\ell}+\max_{\mathsf{u}\in[-u_\infty,u_\infty]}|\sum_{k=1}^{k=d}\mathscr{N}_{2\ell,k}\varphi_k'(\mathsf{u})|}$$
$$=\min\Big(\frac{1}{1-\mathscr{L}_1},\frac{1}{1-\mathscr{L}_2+\max_{\mathsf{u}\in[-u_\infty,u_\infty]}|\sum_{k=1}^{k=d}\mathscr{N}_{2,k}\varphi_k'(\mathsf{u})|},$$
$$\dots,\frac{1}{1-\mathscr{L}_{2W}+\max_{\mathsf{u}\in[-u_\infty,u_\infty]}|\sum_{k=1}^{k=d}\mathscr{N}_{2W,k}\varphi_k'(\mathsf{u})|}\Big).$$

This means that all the BGK segment $\{(\omega,\omega) \text{ s.t. } \omega\in\mathcal{M}_{\text{BGK}}\}$, except its endpoint of largest relaxation parameter, is inside $\mathcal{M}$, thus $\{(\omega,\omega) \text{ s.t. } \omega\in\mathring{\mathcal{M}}_{\text{BGK}}\}\subset\mathring{\mathcal{M}}$.

**SM4. Details of the proof of Theorem 4.10.** For the sake of notation, we understand integration limits and differentials.

$$F=\frac{1}{\Delta t}\iint\sum_{i=1}^{q}\mathcal{R}_i(\boldsymbol{f}_\Delta(t,\boldsymbol{x}))(\psi_\Delta(t,\boldsymbol{x}+\Delta x\boldsymbol{c}_i/\lambda)-\psi_\Delta(t,\boldsymbol{x}))$$
$$+\frac{1}{\Delta t}\iint\Big(\sum_{i=1}^{q}\mathcal{R}_i(\boldsymbol{f}_\Delta(t,\boldsymbol{x}))-u_\Delta(t,\boldsymbol{x})\Big)\psi_\Delta(t,\boldsymbol{x})$$
$$=\lambda\iint\sum_{i=1}^{q}\mathcal{R}_i(\boldsymbol{f}_\Delta(t,\boldsymbol{x}))\frac{\psi_\Delta(t,\boldsymbol{x}+\Delta x\boldsymbol{c}_i/\lambda)-\psi_\Delta(t,\boldsymbol{x})}{\Delta x},$$

where we have used the fact that $\mathsf{u}$ is conserved by the relaxation: $\sum_{i=1}^{q}\mathcal{R}_i(\boldsymbol{f}_\Delta(t,\boldsymbol{x}))-u_\Delta(t,\boldsymbol{x})\equiv 0$. Notice that

$$\frac{\psi_\Delta(t,\boldsymbol{x}+\Delta x\boldsymbol{c}_i/\lambda)-\psi_\Delta(t,\boldsymbol{x})}{\Delta x}\to\frac{1}{\lambda}\sum_{k=1}^{d}c_{i,k}\partial_{x_k}\psi(t,\boldsymbol{x}).$$

We therefore write (understood arguments are $(t,\boldsymbol{x})$)

$$F=\lambda\iint\sum_{i=1}^{q}\mathcal{R}_i(\boldsymbol{f}_\Delta)\Big(\frac{\psi_\Delta(t,\boldsymbol{x}+\Delta x\boldsymbol{c}_i/\lambda)-\psi_\Delta(t,\boldsymbol{x})}{\Delta x}-\frac{1}{\lambda}\sum_{k=1}^{d}c_{i,k}\partial_{x_k}\psi\Big)$$
$$+\iint\sum_{i=1}^{q}(\mathcal{R}_i(\boldsymbol{f}_\Delta)-\mathcal{R}_i(\overline{\boldsymbol{f}}))\sum_{k=1}^{d}c_{i,k}\partial_{x_k}\psi+\iint\sum_{i=1}^{q}(\mathcal{R}_i(\overline{\boldsymbol{f}})-\mathcal{R}_i(\boldsymbol{f}^{\text{eq}}(\overline{u})))\sum_{k=1}^{d}c_{i,k}\partial_{x_k}\psi$$
$$+\iint\sum_{i=1}^{q}(\mathcal{R}_i(\boldsymbol{f}^{\text{eq}}(\overline{u}))-f_i^{\text{eq}}(\overline{u}))\sum_{k=1}^{d}c_{i,k}\partial_{x_k}\psi+\iint\sum_{i=1}^{q}f_i^{\text{eq}}(\overline{u})\sum_{k=1}^{d}c_{i,k}\partial_{x_k}\psi$$
$$=F_1+F_2+F_3+F_4+F_5.$$

Let us discuss each term. For $F_1$, since the terms $\mathcal{R}_i(\boldsymbol{f}_\Delta)$ are uniformly bounded in $\Delta x$ and time-space, because the discrete distribution functions are bounded, we can pass the limit under the integral to obtain $F_1\to 0$. Concerning $F_2$, notice that the functions $\sum_{k=1}^{k=d}c_{i,k}\partial_{x_k}\psi$ are compactly supported and uniformly bounded. Let us

denote by $S$ their largest support and $C > 0$ their largest supremum norm across all $i \in [\![1, q]\!]$. We therefore have

$$0 \leq |F_2| \leq C \iint_S \sum_{i=1}^{q} |\mathcal{R}_i(\boldsymbol{f}_\Delta) - \mathcal{R}_i(\overline{\boldsymbol{f}})| \leq C \iint_S \|\boldsymbol{f}_\Delta - \overline{\boldsymbol{f}}\|_{\ell^1} \to 0,$$

where we use Proposition 4.4 by virtue of the fact that $\boldsymbol{f}_\Delta(t, \boldsymbol{x}) \in K$ a.e. in $\boldsymbol{x}$. Using (4.7) with $T$ large enough and passing to the limit gives the claim. The same idea, taking advantage of the fact that $\overline{\boldsymbol{f}}(t, \boldsymbol{x}) = \boldsymbol{f}^{\text{eq}}(\overline{u}(t, \boldsymbol{x}))$ a.e. in $\boldsymbol{x}$, gives that $F_3 \to 0$. We have $F_4 = 0$ by the simple fact that the equilibria are eigenstates of the relaxation operator with eigenvalue equal to one, so that $\mathcal{R}_i(\boldsymbol{f}^{\text{eq}}(\overline{u})) = f_i^{\text{eq}}(\overline{u})$. We are eventually left with $F_5$.

## REFERENCES

[SM1] D. Aregba-Driollet, *Convergence of Lattice Boltzmann methods with overrelaxation for a nonlinear conservation law*, ESAIM: Mathematical Modelling and Numerical Analysis, 58 (2024), pp. 1935–1958.
